# Supplementary material for: Anomalous and normal dislocation modes in Floquet topological insulators
Source: arXiv:2010.11952 ancillary file (2021-07-23)
Supplement: Supplementary file 1 [file Supplementary_Dislocation_Floquet.pdf]

# Supplementary Information: Anomalous and normal dislocation modes in Floquet topological insulators

Tanay Nag[1] and Bitan Roy[2]

[1]SISSA, via Bonomea 265, 34136 Trieste, Italy

[2]Department of Physics, Lehigh University, Bethlehem, Pennsylvania, 18015, USA

(Dated: October 21, 2020)

## S1. DISLOCATION MODES IN A 2D STATIC TOPOLOGICAL INSULATOR

The Hamiltonian describing a time-reversal symmetry breaking two-dimensional (2D) static topological insulator reads $H = \sum_{\boldsymbol{k}} \Psi^{\dagger}_{\boldsymbol{k}} \, \hat{h}(\boldsymbol{k}) \, \Psi_{\boldsymbol{k}}$, where $\Psi_{\boldsymbol{k}}$ is a two-component spinor and $\hat{h}(\boldsymbol{k}) = \boldsymbol{\sigma} \cdot \boldsymbol{d}(\boldsymbol{k})$, with

$$\boldsymbol{d}(\boldsymbol{k}) = \left( t_1 \sin(k_x a), t_1 \sin(k_y a), m_0 - t_0 \sum_{j=x,y} \cos(k_j a) \right). \tag{S1}$$

Hereafter we set the lattice spacing $a = 1$. As mentioned in the main text that this model supports topological and trivial insulators respectively for $|m_0/t_0| < 2$ and $|m_0/t_0| > 2$. Moreover, within the topological regime there are two distinct insulating phases. Namely, (a) the $\Gamma$ phase, featuring band inversion at the $\Gamma = (0, 0)$ point of the Brillouin zone and (b) the $M$ phase, where the band inversion takes place at the $M = (\pi, \pi)$ point. Respectively, these two phases are found for $0 < m_0/t_0 < 2$ and $-2 < m_0/t_0 < 0$. Here we focus on the $M$ phase. As shown in Fig. S1(a), the corresponding edge modes are indeed found near $k_x = \pi$ in a semi-infinite system with $k_x$ as a good quantum number, but with open boundaries in the $y$ direction.

Next we diagonalize the above Hamiltonian with a pair of edge dislocation-antidislocation and search for the zero-energy modes, bound to the dislocation core in the $M$ phase. To this end, we implement the above tight-binding model in the real space by using the Fourier transformation which in the presence of a single edge dislocation reads

$$\begin{aligned} \hat{h}_{\rm real} = \Bigg( \Bigg[ & \left\{ \left( \sum_{n_x=1}^{\ell_x-2} \sum_{n_y=1}^{\ell_y-1} + \sum_{n_x=\ell_x+1}^{L_x-1} \sum_{n_y=1}^{\ell_y-1} + \sum_{n_x=1}^{L_x-1} \sum_{n_y=\ell_y}^{L_y} \right) c^{\dagger}_{n_x,n_y} c_{n_x+1,n_y} + \sum_{n_y=1}^{\ell_y} c^{\dagger}_{\ell_x-1,n_y} c_{\ell_x+1,n_y} \right\} \otimes \frac{i t_1 \sigma_1 - t_0 \sigma_3}{2} \\ & + \left\{ \left( \sum_{n_x=1}^{\ell_x-1} \sum_{n_y=1}^{L_y-1} + \sum_{n_x=\ell_x+1}^{L_x} \sum_{n_y=1}^{L_y-1} \right) c^{\dagger}_{n_x,n_y} c_{n_x,n_y+1} + \sum_{n_y=\ell_y}^{L_y-1} c^{\dagger}_{\ell_x,n_y} c_{\ell_x,n_y+1} \right\} \otimes \frac{i t_1 \sigma_2 - t_0 \sigma_3}{2} \Bigg] + H.c. \Bigg) \\ & + \sum_{j=1}^{L_x L_y - (\ell_y - 1)} c^{\dagger}_{j,j} c_{j,j} \otimes m_0 \, \sigma_3. \end{aligned} \tag{S2}$$

Here $c_{i,j}$ ($c^{\dagger}_{i,j}$) is the fermion annihilation (creation) operator at site $(i, j)$. In this construction, the center or core of the edge dislocation is located at $(\ell_x, \ell_y)$ [see Fig. 1 of the main text]. This construction can be generalized to implement a pair of edge dislocation-antidislocation with periodic boundaries. In Fig. S1(b) we display the energy spectra in such a system, showing the existence of two modes at (almost) zero energy (red dots), which are well separated from the bulk states (black dots). Furthermore, the spatial profile of the local density of states (LDoS) shows that these two modes are highly localized near the center of the pair of edge dislocation-antidislocation, see Fig. S1(c). Hence, the $M$ phase is translationally active in a 2D static topological insulator. By contrast, the $\Gamma$ phase supports edge modes near $k_x = 0$ and does not lead to any dislocation modes near the zero energy. Whereas in a static trivial insulator there is no edge mode to begin with. We follow the same procedure while scrutinizing the response of any Floquet insulator to dislocation.

## S2. FLOQUET OPERATOR AND FLOQUET HAMILTONIAN

In this section we present details of the Floquet or time evolution operator $U(\boldsymbol{k}, T)$ and the corresponding Floquet Hamiltonian $\hat{h}_{\rm Flq}(\boldsymbol{k})$. When a static system, described by the Hamiltonian $\hat{h}(\boldsymbol{k})$, is periodically driven by the

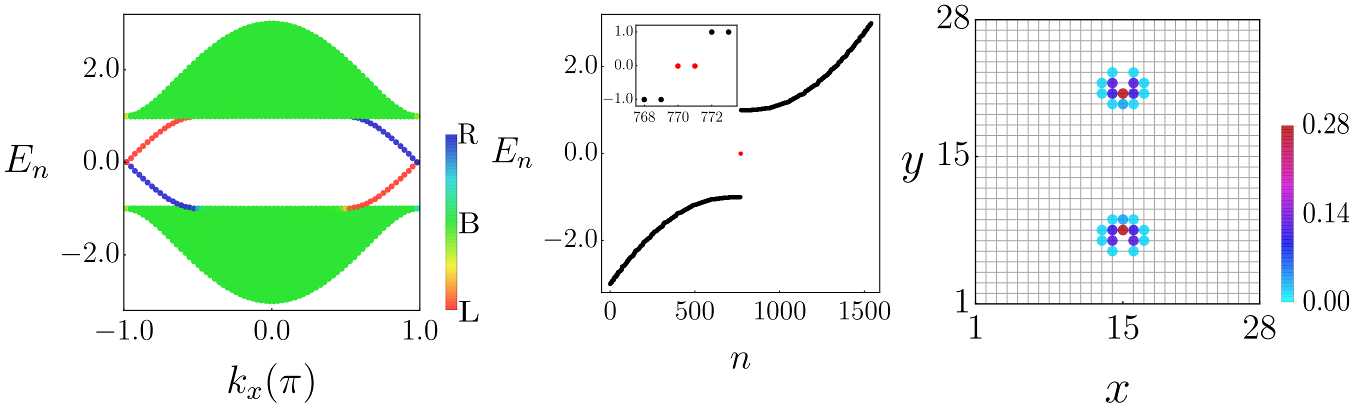


Figure S1: Dislocation as a bulk probe of a static topological insulator with the Chern number $C = 1$. (a) Energy ($E_n$) spectra in a semi-infinite system (with $k_x$ as a good quantum number) of linear dimension $L = 100$ in the $y$ direction (with open boundaries) for $t_1 = t_0 = -m_0 = 1.0$ (yielding the $M$ phase). Here blue and red [green] states are localized on the right (R) and left (L) edges [in the bulk (B)] of the system, respectively, confirming that the band inversion takes place at $k_x = \pi$. (b) The zero energy ($E_n = 0$) dislocation modes (red), well separated from the bulk states (black), in a periodic system with a pair of edge dislocation-antidislocation with the Burgers vector $\mathbf{b} = \pm a\mathbf{e}_x$. (c) Local density of states (LDoS) of the dislocation modes. This situation is qualitatively similar to the FTI with $C = +1$ in the high frequency regime (Fig. 3 of the main text).

perturbation $\hat{V}(t)$ [Eqs. (1) and (3) of main text], the corresponding time evolution operator after a single kick reads

$$U(\boldsymbol{k}, T) = \mathrm{TO}\left(\exp\left[-i\int_0^T \left[\hat{h}(\boldsymbol{k}) + \hat{V}(t)\right] dt\right]\right) = \exp(-im_1\sigma_3)\exp(-i\hat{h}(\boldsymbol{k})T) \equiv \exp\left(-\hat{h}_{\mathrm{Flq}}(\boldsymbol{k})\right). \tag{S3}$$

Here 'TO' stands for time-ordered product. The effective Floquet Hamiltonian $\hat{h}_{\mathrm{Flq}}(\boldsymbol{k}) = \boldsymbol{\sigma}\cdot\boldsymbol{d}_{\mathrm{ren}}(\boldsymbol{k})$, assumes the form of its static counterpart $\hat{h}(\boldsymbol{k})$, however, in terms of the renormalized $d_{\mathrm{ren}}(\boldsymbol{k})$ vector. Explicitly, it reads as $\boldsymbol{d}_{\mathrm{ren}}(\boldsymbol{k}) = d_0(\boldsymbol{k})\boldsymbol{d}'(\boldsymbol{k})$, where

$$\begin{aligned} d_0(\boldsymbol{k}) &= \frac{1}{T}\,\mathrm{Arccos}\Big(A - D\,\frac{d_3(\boldsymbol{k})}{|\boldsymbol{d}(\boldsymbol{k})|}\Big), \quad d_1'(\boldsymbol{k}) = \frac{d_0(\boldsymbol{k})}{\sin(d_0(\boldsymbol{k})T)}\Big(B\,\frac{d_1(\boldsymbol{k})}{|\boldsymbol{d}(\boldsymbol{k})|} - D\,\frac{d_2(\boldsymbol{k})}{|\boldsymbol{d}(\boldsymbol{k})|}\Big), \\ d_2'(\boldsymbol{k}) &= \frac{d_0(\boldsymbol{k})}{\sin(d_0(\boldsymbol{k})T)}\Big(B\,\frac{d_2(\boldsymbol{k})}{|\boldsymbol{d}(\boldsymbol{k})|} + D\,\frac{d_1(\boldsymbol{k})}{|\boldsymbol{d}(\boldsymbol{k})|}\Big), \quad d_3'(\boldsymbol{k}) = \frac{d_0(\boldsymbol{k})}{\sin(d_0(\boldsymbol{k})T)}\Big(B\,\frac{d_3(\boldsymbol{k})}{|\boldsymbol{d}(\boldsymbol{k})|} + C\Big), \end{aligned} \tag{S4}$$

with $|\boldsymbol{d}(\boldsymbol{k})| = \sqrt{d_1^2(\boldsymbol{k}) + d_2^2(\boldsymbol{k}) + d_3^2(\boldsymbol{k})}$ and

$$A = \cos(|\boldsymbol{d}(\boldsymbol{k})|T)\,\cos m_1, \quad B = \sin(|\boldsymbol{d}(\boldsymbol{k})|T)\,\cos m_1, \quad C = \cos(|\boldsymbol{d}(\boldsymbol{k})|T)\,\sin m_1, \quad D = \sin(|\boldsymbol{d}(\boldsymbol{k})|T)\,\sin m_1. \tag{S5}$$

We compute the Chern number $C$ [Eq. (2) of the main text] from the components of the $\boldsymbol{d}_{\mathrm{ren}}(\boldsymbol{k})$ vector to construct the global phase diagram of the time-reversal symmetry breaking Floquet insulators, shown in Fig. 2 of the main text.

## S3. FLOQUET TOPOLOGICAL INSULATORS WITH $C = \pm 1$ AT MEDIUM AND LOW FREQUENCIES

In the high frequency regime ($\omega \gtrsim 8$), as shown in Fig. 2 of the main text, the Floquet insulators can be either topological with $C = \pm 1$ or trivial with $C = 0$. Specifically, the $C = +1$ FTI is qualitatively similar to the one found in a static system [see Sec. S1 and Fig. S1]. For example, it features zero quasienergy normal dislocation modes at the Floquet zone center as the associated Floquet-Bloch band inversion takes place at the $M$ point of the Brillouin zone [see Fig. 3 of the main text]. Moreover, the $C = 0$ Floquet insulator in the high-frequency regime is devoid of any dislocation modes, as in the static system. By contrast, the $C = -1$ FTI supports anomalous dislocation mode at the Floquet zone boundary [see Fig. 3 of the main text], which does not have any analogue in the static system.

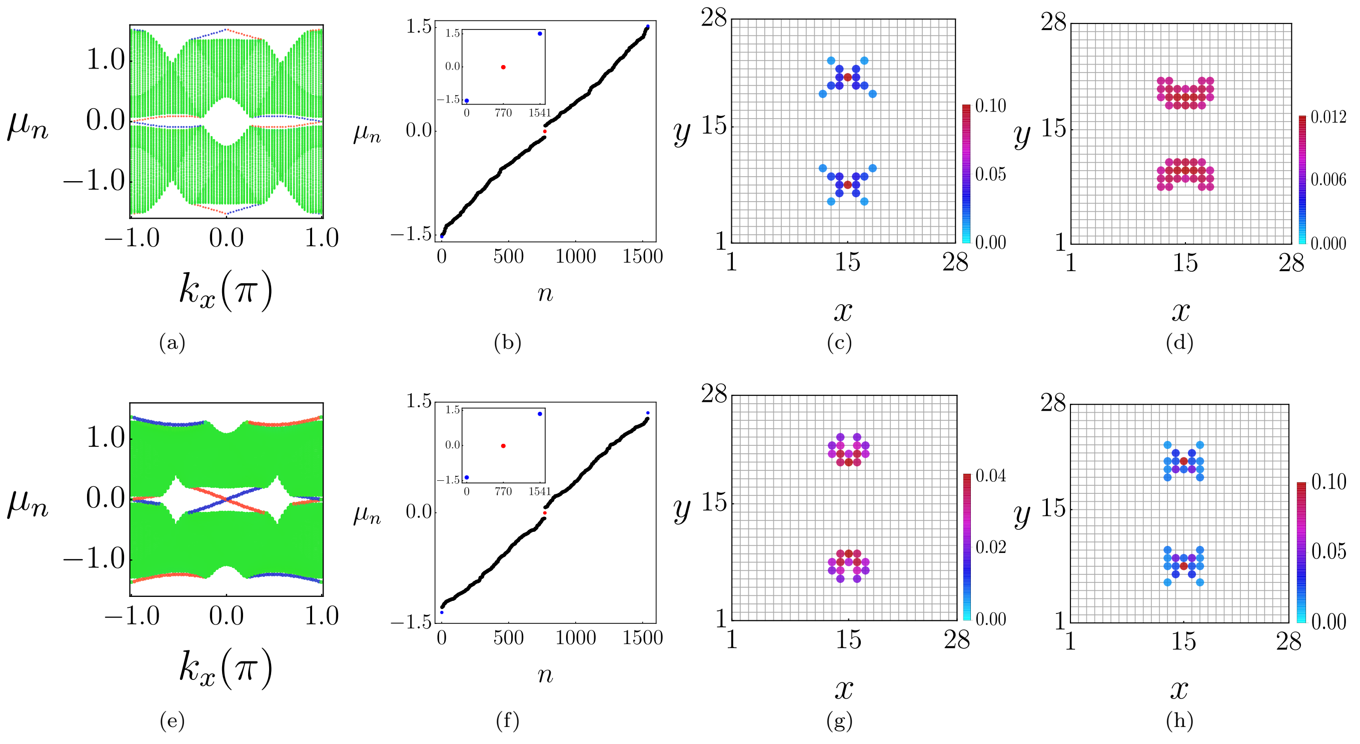


Figure S2: Dislocation as a bulk probe of FTIs with $C=+1$ [(a)-(d)] and $C=-1$ [(e)-(h)] at low frequencies. (a) Quasienergy ($\mu_n$) spectra in a semi-infinite system (with $k_x$ as a good quantum number) of linear dimension $L=100$ in the $y$ direction (with open boundaries) for $\omega=3.05$, $m_1=-7.03$, $t_1=t_0=1.0$ and $m_0=3.0$. Here blue and red [green] states are localized on the right (R) and left (L) edges [in the bulk (B)] of the system, respectively. (b) Normal (red) and anomalous (blue) dislocation modes, separated from the bulk states (black) by finite energy gaps. Corresponding LDoS for the (c) normal and (d) anomalous dislocation modes. Panels (e)-(f) are identical to panels (a)-(d), however for a FTI with $C=-1$ realized for $\omega=2.72$, $m_1=-4.46$, $t_1=t_0=1.0$ and $m_0=3.0$. Colorbars in (a) and (e) are identical to that in Fig. S1(a).

On the other hand, even though in the medium and low frequency regimes, we find the Floquet insulating phases with $C=\pm1$ and 0 [see Fig. 2 of the main text], they are quite different than the ones occupying the high frequency regime. For example, as shown in the main text [see Fig. 5], a Floquet insulator with $C=0$ can feature edge modes at Floquet zone center and boundary at the $\Gamma$ and $M$ points. The edge modes near the $M$ point are ultimately responsible for the normal and anomalous dislocation modes, respectively residing at the Floquet zone center and boundary. The Chern number $C=0$ in such a phase can be reconciled with the fact that in Floquet insulators $C=C_{\rm ZC}-C_{\rm ZB}$, where $C_{\rm ZC}$ ($C_{\rm ZB}$) is the Chern number at the Floquet zone center (boundary). For the above mentioned $C=0$ phase, we find that $C_{\rm ZC}=C_{\rm ZB}=0$, as it features Floquet-Bloch band inversion at both $\Gamma$ and $M$ points at Floquet zone center and boundary. Note that such a $C=0$ Floquet insulator, which we name the $\pi$-trivial insulator, as well as the ones with $C=\pm2$ bear no analogues in static system. Even though we cannot rule out the possibility of a $C=0$ Floquet insulator with $C_{\rm ZC}=C_{\rm ZB}=\pm1$, the model we study here does not show such a phase down to frequency $\omega=1.5$.

The fact that in a time-reversal symmetry breaking Floquet insulator the net Chern number ($C$) accounts for the contributions arising from the Flqouet zone center (yielding $C_{\rm ZC}$) and its boundary (yielding $C_{\rm ZB}$), with $C=C_{\rm ZC}-C_{\rm ZB}$, opens up various possibilities to realize a net $C=\pm1$ FTIs, without any analogues in a static system. Here we discuss two such possibilities, and refer to the phase diagram shown in Fig. 2 of the main text and Fig. S2. Note that a $C=+1$ insulator can be realized when $C_{\rm ZC}=1$ and $C_{\rm ZB}=0$. While $C_{\rm ZC}=1$ results in the edge modes near $k_x=\pi$ at the Floquet zone center, we find edge modes near $k_x=0$ and $\pi$ at the Floquet zone boundary, yielding $C_{\rm ZB}=0$. This situation is demonstrated in Fig. S2(a). According to the $\mathbf{K}\cdot\mathbf{b}$ rule, such as phase then features both normal and anomalous dislocation modes, shown in Fig. S2(b)-(d). The dislocation modes solely arise from the edge modes near $k_x=\pi$. The situation for the $C=-1$ FTI is exactly the opposite [see Fig. S2(e)], which also supports both normal and anomalous dislocation modes, see Fig. S2(f)-(h).
